# Supplementary material for: SPIRE: Semantic Prompt-Driven Image Restoration
Source: arXiv:2312.11595 source file (2024-07-16)
Supplement: Supplementary file 1 [file real-world-supp.tex]

\newcommand{\imgwidth}{0.4\columnwidth}

\begin{figure*}[t]
\centering
% \footnotesize
\setlength\tabcolsep{1pt}
{

\resizebox{1\linewidth}{!}{
\begin{tabular}
{@{}*{7}{c}@{}}
     Input & Ours without semantic prompt & Ours SPIRE Model \\
 \includegraphics[width=\imgwidth]{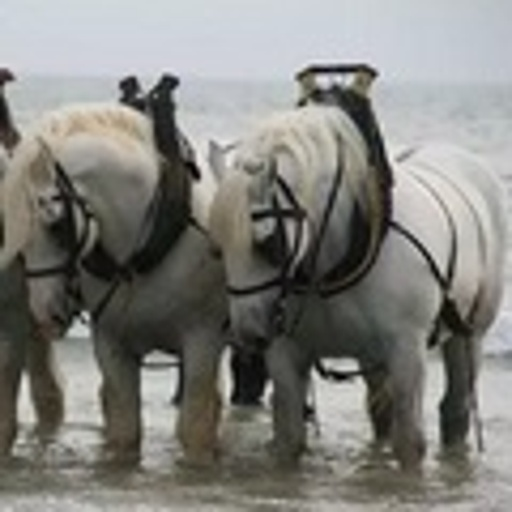} &
     \includegraphics[width=\imgwidth]{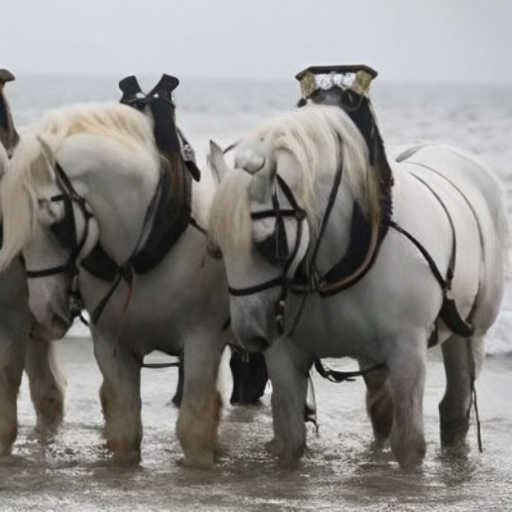} & 
     \includegraphics[width=\imgwidth]{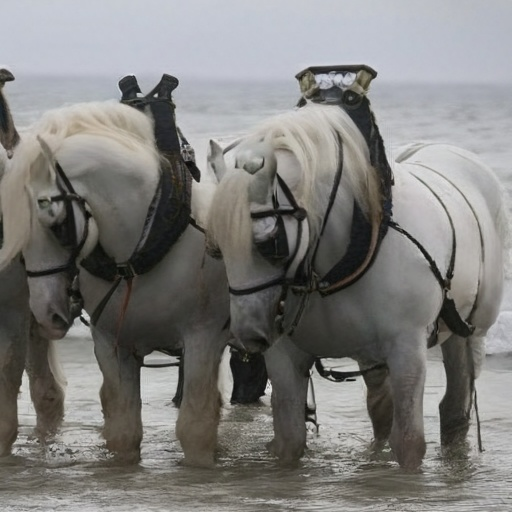}
     \\
     \multicolumn{3}{c}{LLAVA caption: \emph{The image features a group of white horses standing in shallow water...}} 
    
    \\
     \includegraphics[width=\imgwidth]{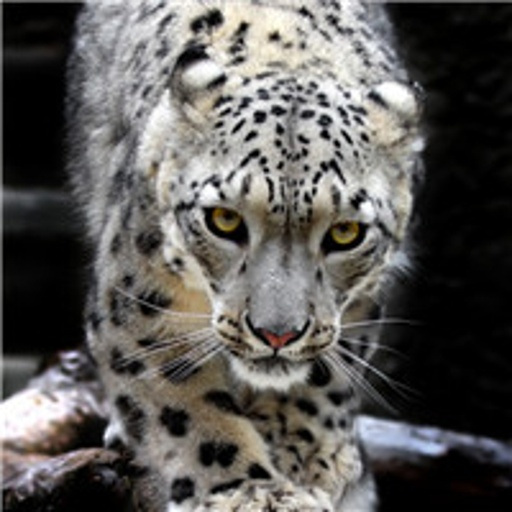} &
     \includegraphics[width=\imgwidth]{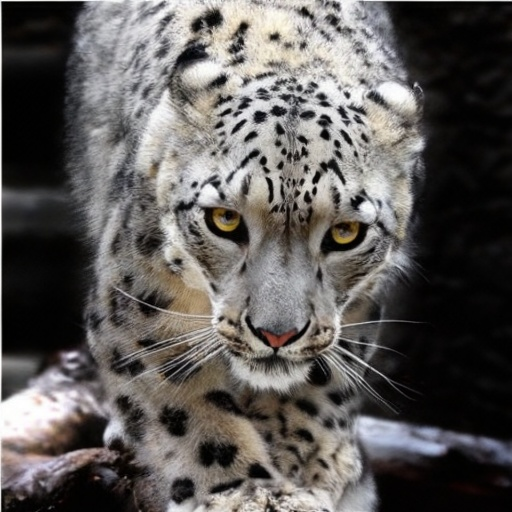} &
     \includegraphics[width=\imgwidth]{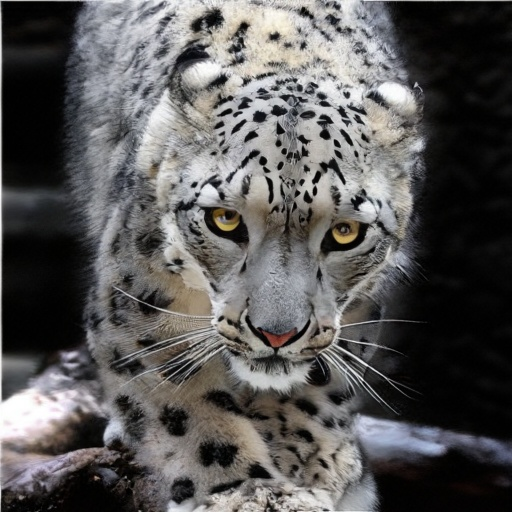} 
     \\
      \multicolumn{3}{c}{LLAVA caption: \emph{The image features a close-up of a snow leopard's face...}} \\
     \\   
     \includegraphics[width=\imgwidth]{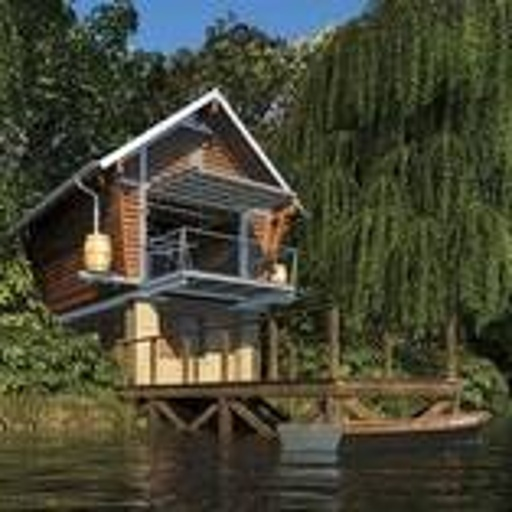} & 
     \includegraphics[width=\imgwidth]{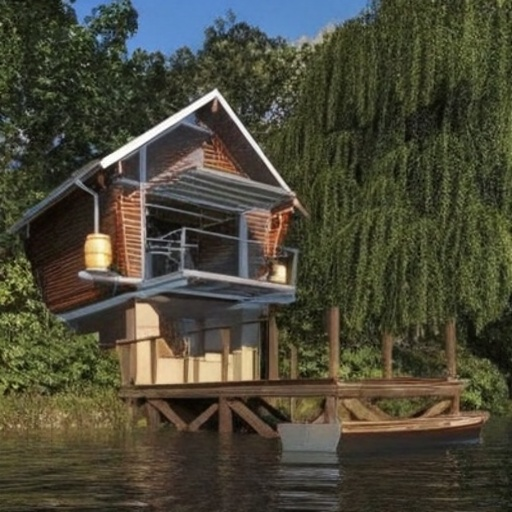} &
     \includegraphics[width=\imgwidth]{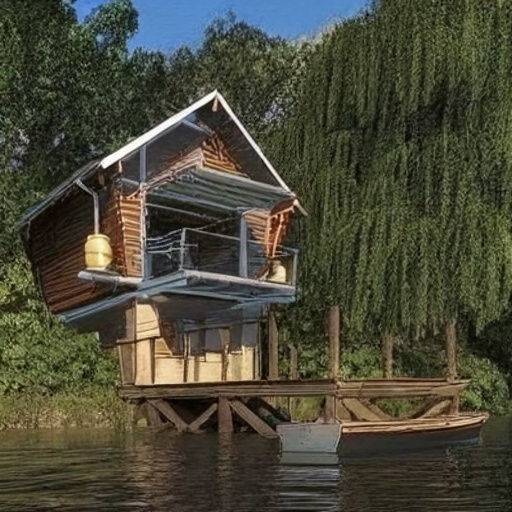} &
     
\\ 
    %  \multicolumn{3}{c}{LLAVA caption: \emph{    
     \multicolumn{3}{c}{LLAVA caption: \emph{The image features a group of white horses standing in shallow water...} } 
\\
     \includegraphics[width=\imgwidth]{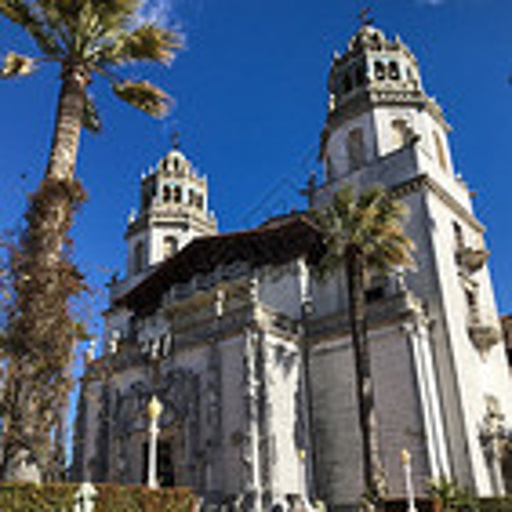} & 
     \includegraphics[width=\imgwidth]{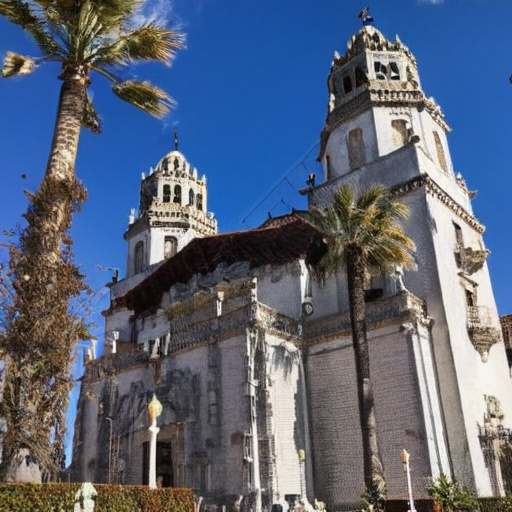} &
     \includegraphics[width=\imgwidth]{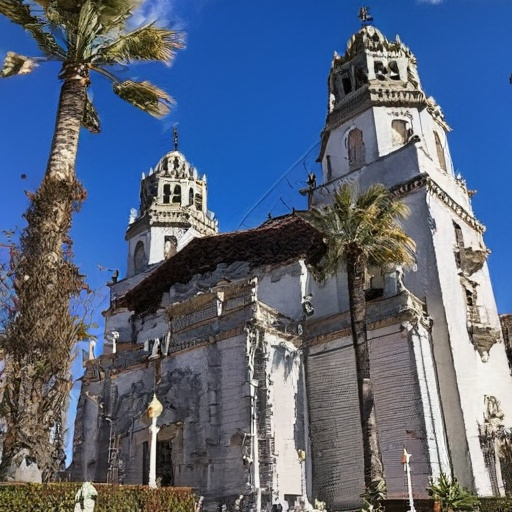} &
\\  
     \multicolumn{3}{c}{LLAVA caption: \emph{The image features a large, ornate church with a clock tower and two towers on top....} } 
\\
     \includegraphics[width=\imgwidth]{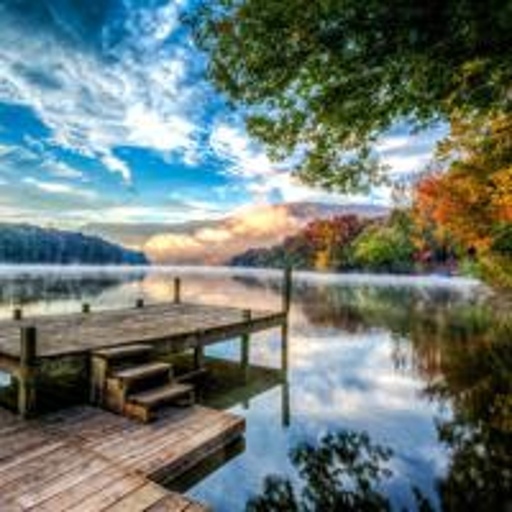} & 
     \includegraphics[width=\imgwidth]{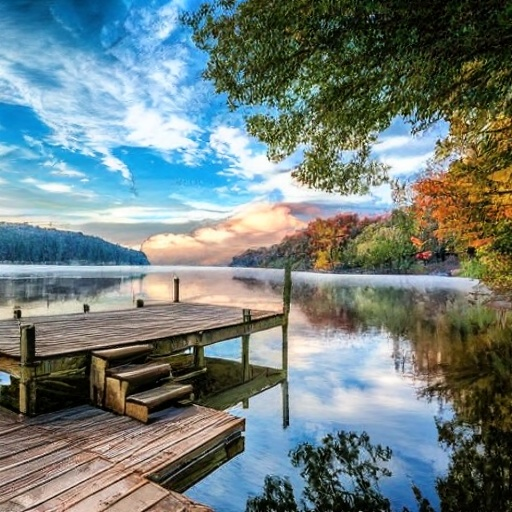} &
     \includegraphics[width=\imgwidth]{sec/figs/supp/real/run0_55_full.jpg} &
\\
     \multicolumn{3}{c}{LLAVA caption: \emph{The image features a serene scene of a dock situated on a lake....} }

\end{tabular}
}
}
\caption{Qualitative comparison on real-world images.}
\label{fig:real-world-visuals-suppl}
\end{figure*}

% \begin{figure*}[t]
% \centering
% % \footnotesize
% \setlength\tabcolsep{1pt}
% {
% \renewcommand{\arraystretch}{0.6}
% \resizebox{1\linewidth}{!}{
% \begin{tabular}{@{}*{7}{c}@{}}
%      Input & Ours without semantic prompt & Ours SPIRE Model \\
%      \includegraphics[width=\imgwidth]{sec/figs/supp/real/18_lq.jpg} & 
%      \includegraphics[width=\imgwidth]{sec/figs/supp/real/run0_18_wo_cs.jpg} &
%      \includegraphics[width=\imgwidth]{sec/figs/supp/real/run0_18_full.jpg} &
     
% \\ 
%     %  \multicolumn{3}{c}{LLAVA caption: \emph{    
%      \multicolumn{3}{c}{LLAVA caption: \emph{The image features a group of white horses standing in shallow water...} } 
% \\
%      \includegraphics[width=\imgwidth]{sec/figs/supp/real/20_lq.jpg} & 
%      \includegraphics[width=\imgwidth]{sec/figs/supp/real/run0_20_wo_cs.jpg} &
%      \includegraphics[width=\imgwidth]{sec/figs/supp/real/run0_20_full.jpg} &
% \\  
%      \multicolumn{3}{c}{LLAVA caption: \emph{The image features a large, ornate church with a clock tower and two towers on top....} } 
% \\
%      \includegraphics[width=\imgwidth]{sec/figs/supp/real/55_lq.jpg} & 
%      \includegraphics[width=\imgwidth]{sec/figs/supp/real/run0_55_full.jpg} &
%      \includegraphics[width=\imgwidth]{sec/figs/supp/real/run0_55_full.jpg} &
% \\
%      \multicolumn{3}{c}{LLAVA caption: \emph{The image features a serene scene of a dock situated on a lake....} } 
% \\
% \end{tabular}
% }
% }
% \caption{Qualitative comparison on real-world images.}
% \label{fig:real-world-visuals-supp2}
% \end{figure*}
